# Supplementary material for: Visual Chirality
Source: arXiv:2006.09512 source file (2020-06-16)
Supplement: Supplementary file 1 [file paperdetails.tex]

\newcommand{\articletitle}{Visual Chirality---Supplemental Material:\\Commutativity and the Chirality of Imaging Processes}

\newcommand{\firstauthor}{}
\newcommand{\firstauthoraffiliation}{}
\newcommand{\firstauthoremail}{}
\newcommand{\firstauthorfootnote}{}
